# Supplementary material for: Aharonov-Bohm Caging and Inverse Anderson transition in Ultracold Atoms
Source: arXiv:2208.02956 source file (2022-08-05)
Supplement: Supplementary file 1 [file ABCage_supplementary_0804.pdf]

# Supplementary Material: Aharonov-Bohm Caging and Inverse Anderson transition in Ultracold Atoms

Hang Li,[1,*] Zhaoli Dong,[1,*] Stefano Longhi,[2,3] Qian Liang,[1] Dizhou Xie,[1,†] and Bo Yan[1,‡]

[1] *Interdisciplinary Center of Quantum Information, State Key Laboratory of Modern Optical Instrumentation, Zhejiang Province Key Laboratory of Quantum Technology and Device, Department of Physics, Zhejiang University, Hangzhou 310027, China*

[2] *Dipartimento di Fisica, Politecnico di Milano, Piazza L. da Vinci 32, I-20133 Milano, Italy*

[3] *IFISC (UIB-CSIC), Instituto de Fisica Interdisciplinar y Sistemas Complejos, Palma de Mallorca, Spain*

## A. Experimental details

The $^{87}Rb$ Bose-Einstein condensate is prepared in a crossed optical dipole trap with a typical atomic number of $2 \times 10^5$. The dipole trap frequencies are $2\pi\times$ (40, 100, 115) $Hz$, , as illustrated in Fig. S1. We adopt the absorption image to detect the atomic population. In experiment, we turn off the optical dipole trap and the Raman-Bragg lasers, then take the absorption image after a 20 $ms$ time-of-flight. In free flight process, atoms with different momentum states will be separated and we can extract the atom population distribution of different momentum states. For constructing the momentum lattice, the Raman-Bragg lasers are imposed along the weak-trapping direction.

For each unit cell (labeled by $n$ in Fig. 1 of main text), we apply two pairs of Raman-Bragg lasers, and there are another two pairs of Raman-Bragg lasers to connect the adjacent unit cells, which is depicted in Fig. S1(b). As Fig. S1shows, each pair of Raman-Bragg lasers has a single-frequency laser (depicted in solid lines) and several

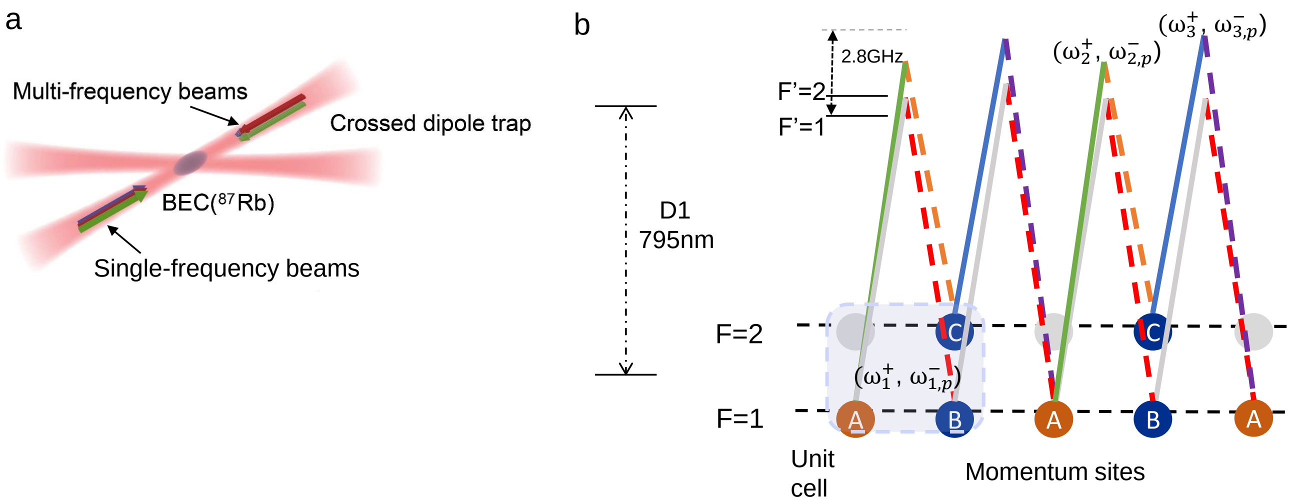


FIG. S1: **a**, The momentum lattice is constructed with three Raman-Bragg laser pairs per unit cell, which are indicated with different colors and labeled by their corresponding frequencies $\{\omega_j^+, \omega_{j,p}^-\}$ $(j = 1, 2, 3)$. **b**, Level schemes for the multi-frequency Raman-Bragg couplings. The solid lines represent the single-frequency lasers (coming from the left in **a**), and the dashed lines represent the multi-frequency lasers (coming from the right in **b**). The unit-cell index $n$ is also illustrated. The couplings between states $\{|n,a\rangle, |n,c\rangle\}$ and $\{|n,b\rangle, |n,c\rangle\}$ are two-photon processes. All the Raman coupling is in the near-resonant condition, whose detuning to the excited energy levels is around 2.8 $GHz$. The hyperfine split between $F = 1$ and $F = 2$ of $^{87}Rb$ is 6.8 $GHz$.

---

*These authors contributed equally to this work
†Current address: Institut für Experimentalphysik und Zentrum für Quantenphysik, Universität Innsbruck, 6020 Innsbruck, Austria
‡Electronic address: yanbohang@zju.edu.cn

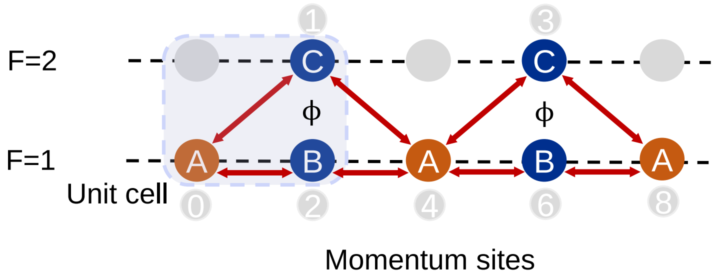


FIG. S2: **The diagram of full Hamiltonian**. The numbers coded in different internal states are classified as follows: the momentum states in $F = 1$ internal state are denoted as even number, while the momentum states in $F = 2$ internal state are denoted as odd number.

multi-frequency lasers (depicted in dashed lines), where these two types of lasers are propagated in opposite directions. While the laser frequencies are given by $\{\omega_j^+, \omega_{j,p}^-\}$ $(j = 1, 2, 3)$, they couple the adjacent momentum states $|p\rangle$ and $|p+1\rangle$ (where $p$ labels the momentum states in units of $2\hbar k$ with $k$ the wave vector of the 795 nm laser, $\pm$ stand for the propagating direction of the beams). Specifically, the $\{\omega_1^+, \omega_{1,p}^-\}$ couples the same internal state, and the $\{\omega_{2/3}^+, \omega_{2/3,p}^-\}$ couple the different internal states. The mapping between the momentum-lattice states with the atomic momentum states can be denoted as

$$|n,a\rangle \;\rightarrow\; |F=1, p=2n\rangle \;\rightarrow\; |g_1, 2(2n)\rangle \tag{1}$$
$$|n,b\rangle \;\rightarrow\; |F=1, p=2n+1\rangle \;\rightarrow\; |g_1, 2(2n+1)\rangle \tag{2}$$
$$|n,c\rangle \;\rightarrow\; |F=2, p=2n+1\rangle \;\rightarrow\; |g_2, 2n+1\rangle \tag{3}$$

Here, the $n$ stands for the $n_{th}$ unit cell. We have used $g_{1/2}$ labels the internal states $F = 1/2$, and the $p$ in second column stands for the real momentum state, as Fig. S2 shows. For the convenience of writing the full hamiltonian of all the interaction processes, we use even numbers to denote the $g_1$ states and odd numbers to denote the $g_2$ states. In this form, the labels $g_{1/2}$ in the third column can also be removed.

Under such a mapping, lasers with frequencies $\{\omega_1^+, \omega_{1,p}^-\}$ couple momentum states in the same internal state.

$$\text{two photon process}: \quad |n,a\rangle \leftrightarrow |n,b\rangle \;\text{ with }\; \omega_{1,p}^- = \omega_1^+ - (4n+1)4E_r/\hbar, \tag{4}$$
$$|n,b\rangle \leftrightarrow |n+1,a\rangle \;\text{ with }\; \omega_{1,p}^- = \omega_1^+ - (4n+3)4E_r/\hbar. \tag{5}$$

Lasers with frequencies $\{\omega_2^+, \omega_{2,p}^-\}$ couple $|n,a\rangle \leftrightarrow |n,c\rangle$, in two-photon processes with frequencies

$$\omega_{2,p}^- = \omega_2^+ - \Delta_{\text{hyp}} - (4n+1)4E_r/\hbar. \tag{6}$$

Here $\Delta_{\text{hyp}}$ is the hyperfine splitting between the ground state manifolds $F = 1$ and $F = 2$.

Finally, lasers with $\{\omega_3^+, \omega_{3,p}^-\}$ couple $|n,c\rangle \leftrightarrow |n,b\rangle$, in two-photon processes with frequencies

$$\omega_{3,p}^- = \omega_3^+ + \Delta_{\text{hyp}} + (4n+3)4E_r/\hbar. \tag{7}$$

The Fig.1(a) and the effective hamiltonian $H_{eff}$ of the main text give the ideal configuration of the AB cage. However, the actual experiment can not realize perfect manipulation. On the one hand, we set the four adjacent tunneling process with the same 1 $kHz$ Rabi coupling, but the real-life controlling has slightly unsymmetry.The actual experimental parameters of this four neighboring coupling is $(0.95(5)kHz$ ,$0.97(5)kHz$ ,$0.96(5)kHz$ ,$0.95(5)kHz)$. On the other hand, although we have adopt near-resonant coupling with only 2.8 $GHz$ for prohibiting coupling all the adjacent momemtum states in the $F = 2$ energy level, the actual experiment still has weak coupling in the lattice site of $F = 2$ level with around $1/4$ times as the coupling in $F = 1$ level. The above imperfect manipulation of our experiments leads to the leakage of AB cage dynamics in the Fig.2 and 3.

### B. The full Hamiltonian of synthetic momentum lattice

The ideal Hamiltonian has been written in the equation (1) of main text, which mainly takes the resonant coupling of adjacent sites into considerations. Through adiabatically eliminating the excited states (assume that the one-photon

detuning is relatively small here), we can write out the full Hamiltionian of this scheme [1, 2]. For simplicity, the far-resonant terms are neglected here.

$$H_{full} = \sum_n \sum_i [\frac{\hbar\tilde{\Omega}_i^1}{2} e^{i(\delta_i^1 t-\phi_i^1)} e^{-i(2n+1)4E_r t/\hbar} |g_1, 2n\rangle \langle g_1, 2(n+1)| + \frac{\hbar\tilde{\Omega}_i^2}{2} e^{i(\delta_i^2 t-\phi_i^2)} e^{-i(4n+1)4E_r t/\hbar} |g_1, 2(2n)\rangle \langle g_2, 2n+1|$$
$$+ \frac{\hbar\tilde{\Omega}_i^3}{2} e^{i(\delta_i^3 t-\phi_i^3)} e^{-i(4n+3)4E_r t/\hbar} |g_2, 2n+1\rangle \langle g_1, 2(2(n+1))| + h.c.] \tag{8}$$

where the $\tilde{\Omega}_i^1 = \frac{\Omega_+^1 \Omega_{-,i}^1}{2\Delta_1}, \tilde{\Omega}_i^2 = \frac{\Omega_+^2 \Omega_{-,i}^2}{2\Delta_2}$ and $\tilde{\Omega}_i^3 = \frac{\Omega_+^3 \Omega_{-,i}^3}{2\Delta_3}$ are the effective Rabi frequencies (here the subscript $i$ implies that we should consider the coupling of all the multi-frequencies beams rather than the single pair of resonant Raman coupling between each pair of momentum states), $\Delta_i$ $(i = 1, 2, 3)$ is the corresponding one-photon detuning, $\Omega_+^n$ is the Rabi frequency of the $n_{th}$ laser propagating at + direction and $\Omega_{-,i}^n$is the Rabi frequency of the $i_{th}$ frequency intensity of the $n_{th}$ beam that propagation at - direction. $\delta_i^n = (\omega_+^n - \omega_+^0) - (\omega_{-,i}^n - \omega_{-,i}^0)$ is the two-photon detuning of the paired $n_{th}$ (n=1,2,3) beam ($\omega_\pm^0$ are the resonant frequencies). $\phi_i^n = \phi_+^n - \phi_{-,i}^n$ is the phase difference of the paired $n_{th}$ (n=1,2,3) beam. The synthetic magnetic flux can be defined as $\phi_i = 2\phi_i^1 + \phi_i^2 + \phi_i^3$.

### C. Single-particle energy spectrum and inverse Anderson transition

In the single-particle sector of Hilbert space, we may set $|\psi\rangle = \sum_n \left( A_n \hat{a}_n^\dagger + B_n \hat{b}_n^\dagger + C_n \hat{b}_n^\dagger \right) |0\rangle$ for the state vector of the system, with $\sum_n (|A_n|^2 + |B_n|^2 + |C_n|^2) = 1$. Correspondingly, the stationary Schrödinger equation $H_{\rm eff}|\psi\rangle = E|\psi\rangle$ yields the following eigenvalue problem

$$EA_n = -\Delta_n^{(a)} A_n - J(B_n + B_{n-1}) - JC_{n-1} - J\exp(i\phi)C_n \tag{9}$$
$$EB_n = -\Delta_n^{(b)} B_n - J(A_n + A_{n+1}) \tag{10}$$
$$EC_n = -\Delta_n^{(c)} C_n - JA_n \exp(-i\phi) - JA_{n+1} \tag{11}$$

for the energy $E$, where for the sake of definiteness we assumed the gauge $\theta_1 = \phi$ and $\theta_2 = \theta_3 = \theta_4 = 0$. Provided that $E \neq \Delta_n^{(b,c)}$, we can eliminate the amplitude probabilities $B_n$ and $C_n$ from Eqs.(9,10,11),

$$B_n = -J\frac{A_n + A_{n+1}}{E + \Delta_n^{(b)}}\ ,\ \ C_n = -J\frac{A_n \exp(-i\phi) + A_{n+1}}{E + \Delta_n^{(c)}}\ , \tag{12}$$

yielding the following eigenvalue equation for the amplitudes $A_n$

$$EA_n = J_n(E)A_{n+1} + J_{n-1}^*(E)A_{n-1} + V_n(E)A_n. \tag{13}$$

In Eq.(13), the effective energy-dependent hopping amplitudes $J_n(E)$ and on-site potential $V_n(E)$ are given by

$$J_n(E) = J^2 \left( \frac{1}{E + \Delta_n^{(b)}} + \frac{\exp(i\phi)}{E + \Delta_n^{(c)}} \right) \tag{14}$$
$$V_n(E) = -\Delta_n^{(a)} + J^2 \left( \frac{1}{E + \Delta_{n-1}^{(b)}} + . \frac{1}{E + \Delta_n^{(b)}} + \frac{1}{E + \Delta_{n-1}^{(c)}} + \frac{1}{E + \Delta_n^{(c)}} \right). \tag{15}$$

Formally, Eq.(13) can be regarded as the 1D Anderson model with correlated and energy-dependent disorder in both hopping amplitudes and on-site potential. Hence, we expect rather generally Anderson localization to arise in the disordered 1D AB caging system under sufficiently strong disorder.

To unveil the occurrence of an inverse Anderson transition, i.e. a transition from an insulating to a metallic phase, let us focus our attention to the fully flat band case, i.e. $\phi = \pi$, so that in the disorder-free case all eigenstates are compact localized modes and the system is in the insulating phase. Following Ref.[3], let us assume $\Delta_n^{(a)} = 0$ and correlated on-site potential disorder in sublattices B and C, which can be either symmetric or antisymmetric.

For symmetric correlated disorder, we have $\Delta_n^{(c)} = \Delta_n^{(b)} = \Delta_n$, with $\Delta_n$ stochastic independent variables with the same probability density distribution $f(\Delta)$ of zero mean. In this case, according to Eq.(14) with $\phi = \pi$ the hopping amplitudes $J_n(E)$ identically vanish, and thus the eigenstates are still compact localized modes. The corresponding eigenenergies are obtained from the roots of the cubic equation $E = V_n(E)$ with $V_n(E) = 2J^2[1/(E + \Delta_n) + 1/(E +$

$\Delta_{n-1})]$, and they depend on the values of $\Delta_n$. Hence the effect of symmetric correlated disorder in sublattices B and C is to remove eigenvalue degeneracy of the flat band system, but localization in the form of compact modes is preserved.

For the antisymmetric correlated disorder, $\Delta_n^{(c)} = -\Delta_n^{(b)} = \Delta_n$, an inverse Anderson transition can be instead observed. In fact, in this case one has

$$J_n(E) = -J^2 \frac{2\Delta_n}{E^2 - \Delta_n^2} \;\; , \quad V_n(E) = 2EJ^2 \left( \frac{1}{E^2 - \Delta_n^2} + \frac{1}{E^2 - \Delta_{n-1}^2} \right). \tag{16}$$

As shown in [3], since $V_n(E = 0) = 0$ the Layounov exponent at $E = 0$ can be computed analytically and it always vanishes, indicating that the energy $E = 0$ belongs to the energy spectrum of $H_{\rm eff}$ and corresponds to either an extended or a critical state. The existence of extended states suggests that transport in the system induced by disorder is allowed, i.e. that an inverse Anderson transition occurs under correlated anti-symmetric disorder. The kind of transport depends sensitively on the specific form of the distribution function $f(\Delta)$ of disorder, and localization is asymptotically observed when $f(\Delta)$ approaches the uniform distribution [3]. A simple and exactly-solvable case showing inverse Anderson transition, which we implemented in our experiment, is the one corresponding to a Bernoulli distribution, i.e. $\Delta_n$ can take randomly only two values, $\Delta$ or $-\Delta$, with probabilities $p$ and $(1 - p)$. In this case, the effective 1D Anderson model [Eq.(13)] takes the simple form

$$EA_n = -\kappa \left( A_{n+1} \exp(i\varphi_n) + A_{n-1} \exp(-i\varphi_{n-1}) \right) + VA_n \tag{17}$$

where we have set $\kappa = 2J^2\Delta/(E^2 - \Delta^2)$, $V = 4EJ^2/(E^2 - \Delta^2)$ and $\varphi_n = 0$ for $\Delta_n = \Delta$, $\varphi_n = \pi$ for $\Delta_n = -\Delta$. Note that in Eq.(17) disorder enters solely in the Peierls' phase $\varphi_n$ of the hopping amplitude, which can be removed after the gauge transformation

$$A_n = a_n \exp\left( -i \sum_{l}^{n-1} \varphi_l \right) \tag{18}$$

yielding the disorder-free tight-biding lattice model

$$Ea_n = -\kappa \left( a_{n+1} + a_{n-1} \right) + Va_n. \tag{19}$$

Hence, for antisymmetric correlated disorder with the Bernoulli distribution the single-particle energy spectrum of $H_{\rm eff}$ is purely absolutely continuous and formed by three dispersive Bloch bands, as shown in Fig.4(a) of the main manuscript, with the dispersion relations $E = E(k)$ implicitly defined by the relation

$$E(k) = -\frac{4J^2\Delta \cos k}{E^2(k) - \Delta^2} + \frac{4J^2 E(k)}{E^2(k) - \Delta^2} \tag{20}$$

where $-\pi \leq k < \pi$ is the Bloch wave number. The width $\Delta E$ of the absolutely continuous spectrum, defined as the sum of the widths of the three dispersive Bloch bands, vanishes for $\Delta = 0$, i.e., in the limit of the clean AB flatband system, and in the strong disorder limit $\Delta \gg J$. The largest bandwidth is attained at $\Delta = \Delta_0 = \sqrt{2}J$, at which the two gaps separating the three bands close. At this turning point, the transport in the lattice induced by disorder is fastest.

### D. Finite size effects and turning point of disorder strength

As shown in previous section, the fastest transport in the lattice under correlated antisymmetric disorder with a Bernoulli distribution should be observed at the disorder strength $\Delta = \sqrt{2}J$, i.e. at the turning point where the absolutely continuous spectrum of dispersive bands is widest. This theoretical result neglects finite-size (edge) effects of the system and assumes a long observation time of the wave packet dynamics. As discussed in the main text, in our experiment we observed the fastest transport at a higher values of disorder $\Delta$ than the one predicted theoretically. Such a deviation can be mainly ascribed to the finite-size effects of our system, i.e. the relatively short observation time of the dynamics required to avoid edge effects, and to the deviations of the full Hamiltonian $H_{\rm full}$ from the effective one $H_{\rm eff}$.

We have numerically calculated the evolution of the distance $\mathcal{D}(t)$ (defined in the main text) for different observation times $t$ and chain size, assuming open boundary conditions, so as to unravel finite-edge effects and the role of

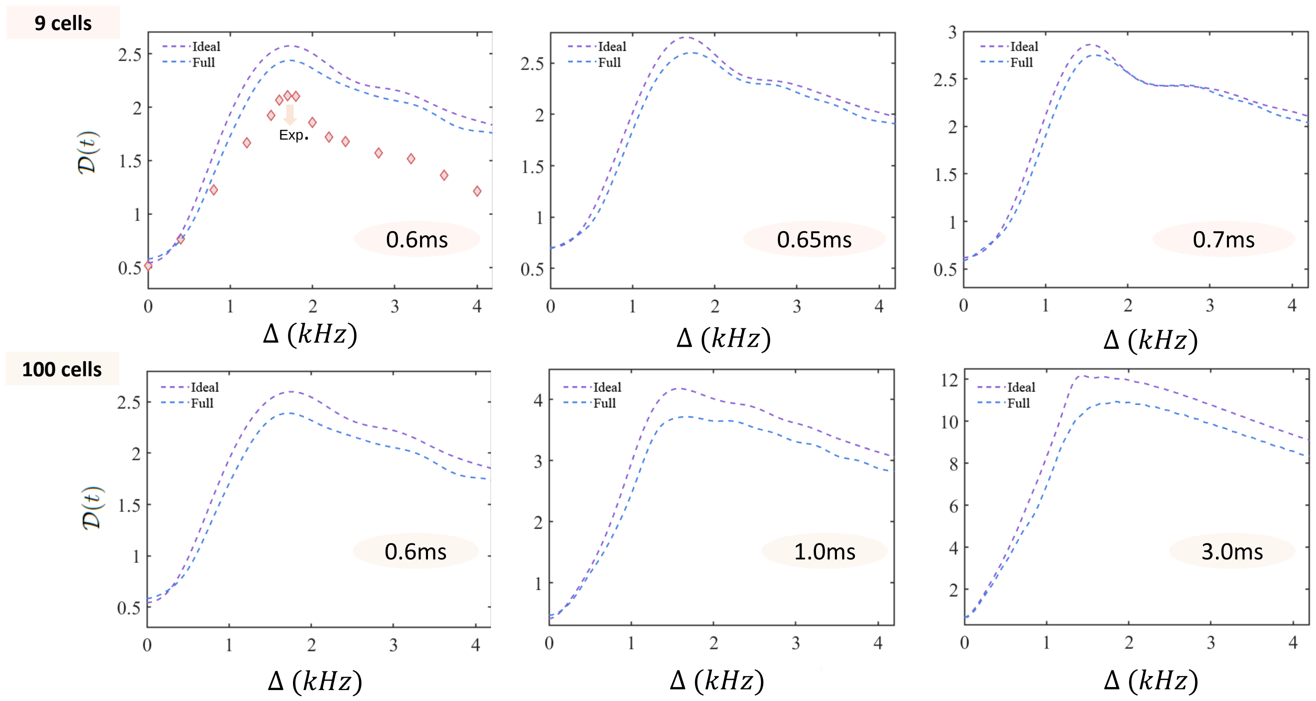


FIG. S3: **Spreading dynamics versus disorder strength for antisymmetric disorder with a Bernoulli distribution in a finite AB chain.** The panels show the numerically-computed distance $\mathcal{D}(t)$, at a few observation times (labelled in the figures), versus disorder strength $\Delta$. Two finite AB lattice chains are considered, comprising either 9 unit cells (upper panels) and 100 unit cells (lower panels). The two dashed curves in each panel, plotted with different colors, refer to the evolution dynamics as obtained using either the effective or the full Hamiltonian. The effective coupling amplitude used in the numerical simulations is the same as in the experiment ( $J = 0.95kHz$).

observation time. The results, shown in Fig.S3, are obtained by evolving the system using either $H_{\text{eff}}$ or $H_{\text{full}}$. The figure clearly shows that the turning point of disorder strength is consistent with the theoretical prediction when we consider a sufficiently long chain to avoid edge effects, and thus a sufficiently long observation time, and when the dynamics is computed using the effective Hamiltonian $H_{\text{eff}}$. For example, for the $t = 3$ ms time evolution in a lattice comprising 100 unit cells, the turning point of disorder in the case of the ideal (effective) Hamiltonian is around 1.45 times the effective coupling amplitude, in agreement with the theoretically-predicted factor $\sqrt{2}$, while in the case of full Hamiltonian a more smooth turning trends is observed. Therefore, our setup and measurement method, adopting the average spreading velocity within a relatively short time to avoid edge effects, can provide a qualitative trend of the bandwidth $\Delta E$ of dispersive bands versus the disorder strength $\Delta$, but cannot detect accurately the position of the turning point.

[1] B. Gadway, *Phys. Rev. A* **92**, 043606 (2015)
[2] E. J. Meier, F. A. An, and B. Gadway, *Phys. Rev. A* **93**, 051602 (2016)
[3] S. Longhi, *Opt. Lett.* **46**(12), 2872-2875 (2021).
